# Supplementary material for: Template-Based Financial Report Generation in Agentic and Decomposed Information Retrieval
Source: arXiv:2504.14233 source file (2025-04-19)
Supplement: Supplementary file 1 [file 7-appendix.tex]

\section{Appendix}

\subsection{Prompts in AgenticIR}
As shown in Table \ref{tab:agent_prompt}, we provided the detailed system prompts used in AgenticIR. These prompts define the role descriptions for each agent. 
Additionally, the User Agent in the task\_decompose function is only responsible for forwarding complex tasks, so its system prompt is set to the default prompt: \textit{You are a helpful AI assistant.}
Furthermore, in the experiment, the prompts used for communication between the agents are generated autonomously by the agents themselves.
% \begin{table*}
% \small
% \caption[c]{System Prompts in AgenticIR}
% \begin{tabular}{l|l}
% \toprule
% Agent & System Prompts \\
% \midrule
% Generate & \makecell[l]{You are a helpful AI Assistant.
% You can interact with Assistant to complete the task.
% Reply 'TERMINATE' if\\ all sub-tasks are completed.}\\
% \midrule
% Assistant Agent &  \makecell[l]{You are a helpful AI assistant.
% You can use the task planner to decompose a complex task into sub-tasks.
% You\\ can also use the retrieve data to get earnings call transcript by subqueries you generate based on sub-tasks.\\
% Make sure to follow through with the subqueries.
% Follow the template to generate the financial report in text\\ format. 
% Add or Return 'TERMINATE' only if the final report is completed.}\\
% \bottomrule
% \end{tabular}
% \label{tab:agent_prompt}
% \end{table*}

\begin{table*}
% \small
\centering
\caption[c]{System Prompts of AgenticIR.}
% \setlength{\tabcolsep}{2.5pt}
% \renewcommand{\arraystretch}{0.9}
% \begin{tabular}{l|p{0.85\textwidth}}
\begin{tabular}{l|l}
% \begin{longtable}{l|p{12cm}}
\toprule
% \cmidrule{2-5}
Agent & System Prompts \\
\midrule
User Proxy Agent & \makecell[l]{You are a helpful AI Assistant.
You can interact with Assistant to complete the task.
Reply\\ 'TERMINATE' if all sub-tasks are completed.}\\
\midrule
Assistant Agent &  \makecell[l]{You are a helpful AI assistant.
You can use the task planner to decompose a complex task into\\ sub-tasks.
You can also use the retrieve data to get earnings call transcript by subqueries you\\ generate based on sub-tasks.
Make sure to follow through with the subqueries.
Follow the template\\ to generate the financial report in text format. 
Add or Return 'TERMINATE' only if the final report\\ is completed.}\\
\midrule
Financial Retrieval Agent & You are financial retriever, a content retrieval assistant.
Retrieve financial data from external resources.\\
\midrule
Financial Manager & You are the financial manager. Your responsibility is to answer the question given the retrieved context.\\
\midrule
Task Decompose Agent & \makecell[l]{You are a helpful AI assistant. 
You suggest a feasible plan for finishing a complex task by\\ decomposing it into lots of sub-tasks.}\\
\bottomrule
\end{tabular}
% \end{longtable}
\label{tab:agent_prompt}
\end{table*}

\subsection{Prompts in DecomposedIR}
In Table \ref{tab:decomposed_prompt}, we presented the LLM prompts used during the generation and summarization process. 
In the generate action, \textit{context} refers to the three relevant chunks from the earnings call transcript, \textit{statement} represents the financial statements, and \textit{question} refers to the decomposed sub-query. 
In the summarize action, \textit{question and answer} denotes the pairs of sub-query and corresponding answers, while \textit{section} refers to a specific section in the report template.
\begin{table*}
% \small
\centering
\caption[c]{LLM Prompts in DecomposedIR.}
% \setlength{\tabcolsep}{2.5pt}
% \renewcommand{\arraystretch}{0.9}
% \begin{tabular}{l|p{0.85\textwidth}}
\begin{tabular}{l|l}
% \begin{longtable}{l|p{12cm}}
\toprule
% \cmidrule{2-5}
Action & LLM Prompts \\
\midrule
Generate & \makecell[l]{You are a senior financial analyst. Based on the provided context (earnings call transcript) and financial\\
statement JSON, try  to answer the question and the numerical value as precise as possible based on\\ the provided context. Ensure clarity and CONCISENESS in the response.\\
Transcript Relevant Context:\\
\textit{\{context\}}\\
Financial Statement JSON:\\
\textit{\{statement\}}\\
Question:\\
\textit{\{question\}}}\\
\midrule
Summarize &  \makecell[l]{I will provide several questions along with their corresponding answers and the reasoning behind those answers,\\
as well as the section to summarize. Please summarize the answers into a single cohesive response focused on\\
this aspect, and consolidate the reasoning into a concise explanation. Ensure that all numerical data is accurately\\ 
preserved and aligned with the section. Do not include any external or speculative information.
The final\\
summarized response and explanation must be logically consistent, focused on the section, and aligned with\\
the provided content.\\
Questions and Answers:\\
\textit{\{question and answer\}}\\
Section to Summarize\\
\textit{\{section\}}\\
}\\
\bottomrule
\end{tabular}
% \end{longtable}
\label{tab:decomposed_prompt}
\end{table*}
